# Supplementary material for: SoK: Analysis of Root Causes and Defense Strategies for Attacks on Microarchitectural Optimizations
Source: arXiv:2212.10221 source file (2022-12-20)
Supplement: Supplementary file 1 [file section8_appendix.tex]

\appendix
\section{Systematization of attacks}
\label{attacks_appendix}
\subsection{Non-transient attacks}
\subsubsection{Cache compression}
